# Supplementary material for: Viscoelastic scaling regimes for marginally-rigid fractal spring networks
Source: arXiv:2201.05391 ancillary file (2022-06-10)
Supplement: Supplementary file 1 [file suppInf.pdf]

## Supplementary materials

**Viscoelastic scaling regimes for fractal marginally–rigid spring networks**

D.A. Head

# S1 Example networks

Examples of networks of $2^n \times 2^n$ nodes with $n = 6$, larger than but otherwise the same as the $n = 4$ examples given in Fig. 1(b) of the main text, are provided as image files in JPEG format with the filename convention `eg_n6_m1.jpg` for $m = 1$, and similarly for $m = 2$ up to and including $m = 6$.

# S2 Derivation of numbers of nodes and bonds

Consider first a single triangle with $2^m$ nodes along each edge that is generated recursively as per the standard Sierpinski triangle, and denote the number of nodes and bonds/springs by $N^m_{\rm node}$ and $N^m_{\rm spring}$ respectively. For $m = 0$, *i.e.* a simple triangle, $N^0_{\rm node} = N^0_{\rm spring} = 3$. Now proceed inductively. Each new iteration can be viewed as taking the original triangle, halving all lengths, and stacking 3 copies to give a new triangle with an inverted triangular 'void' region in the middle. The number of bonds is therefore tripled at each iteration by virtue of repeating the same triangle 3 times, so $N^{m+1}_{\rm spring} = 3N^m_{\rm spring}$ and $N^m_{\rm spring} = 3^{m+1}$. The number of nodes will also triple, except that now 3 must be subtracted to avoid double-counting nodes midway along the larger triangle edges. Thus $N^{m+1}_{\rm node} = 3\,(N^m_{\rm node} - 1)$, which can be shown by induction to satisfy

$$N^m_{\rm node} = \frac{3}{2}\,(3^m + 1)\,. \tag{S1}$$

Now consider the full problem with $n \geq m$. There are $2^{n-m}$ of the major triangles just described along each of the $x$ and $y$–directions. The total number of major triangles is thus $2 \times 2^{n-m} \times 2^{n-m} = 2^{2(n-m)+1}$, where the additional factor of 2 accounts for the two triangles in each rectangular region of nodes. The number of bonds is $2^{2(n-m)+1}$ multiplied by $N^m_{\rm spring} - 3 \times 2^m$, which includes subtraction of bonds along the edges of the major triangles as per the generation algorithm described in the main text. The total number of bonds is therefore

$$N_{\rm spring} = 6\,(3^m - 2^m)\,4^{n-m}. \tag{S2}$$

Note this is zero for $m = 0$, as it should be — there will be no bonds after removal of edges of the major triangles with edge length $2^m = 2^0 = 1$. This is why $m = 1$ is regarded in the main text as the small–$m$ limit, as $m = 0$ generates no network at all.

The bare number of nodes will be $2^{2(n-m)+1}N^m_{\rm node}$, but we must avoid double counting edge nodes, and must now additionally avoid over–counting corner nodes. Returning to the major triangle described above with $N^m_{\rm node}$ nodes, 3 of these are corner nodes and $3\,(2^m - 1)$ are edge (but not corner) nodes, leaving $\frac{3}{2}(3^m + 1) - 3 \cdot 2^m$ internal nodes. For $m < n$, the vertices of the major triangles are entirely removed. Therefore we weight internal nodes by 1 and edge nodes by $\frac{1}{2}$ to give

$$N^{m<n}_{\rm spring} = 2^{2(n-m)+1}\left[\frac{3}{2}(3^m + 1) - 3 \cdot 2^m + \frac{1}{2} \cdot 3 \cdot (2^m - 1)\right] = 3\,(3^m - 2^m)\,4^{n-m}. \tag{S3}$$

For $m = n$, two vertex nodes in total survive because they intersect with the middle of the base of another major triangle (in fact, the same one through the periodic boundaries) rather than a vertex node. Since each such node belongs to two triangles, they should be weighted by a factor $\frac{1}{2}$. Thus (S3) needs to be incremented by $2 \times \frac{1}{2} = 1$ for $n = m$, giving the final expression

$$N_{\rm node} = 3\left(3^m - 2^m\right)4^{n-m} + \delta_{nm} \tag{S4}$$

valid for all $1 \leq m \leq n$, with $\delta_{nm} = 1$ for $n = m$ and 0 otherwise the usual Kronecker delta.

# S3 Derivation of the affine prediction $G'_{\rm aff}$

To derive the affine storage modulus ignoring small corrections due to node perturbations, first note that the affine prediction for a full, regular triangular lattice is

$$G'_{\rm aff,full} = \frac{\sqrt{3}}{4}k \quad . \tag{S5}$$

This standard result can be readily derived by calculating the extension of springs in a unit cell under the assumption of affine deformation, *i.e.* when all nodes move as per the macroscopic shear strain of magnitude $\gamma$, evaluating the elastic energy $E$, and then dividing by the area $A$ of that unit cell. The shear modulus can then be extracted using $\frac{E}{A} = \frac{1}{2}G'_{\rm aff}\gamma^2$. Note that elastic moduli have units of force divided by length in two–dimensions, which is the same as the spring constant, so the above expression is dimensionally correct.

Since the networks generated as described in the main text remain isotropic, *i.e.* have equal numbers of springs of each of the three orientations, the affine prediction is simply that for full triangular lattices (S5) scaled by the fraction of springs that remain in the fractal network. For a system of $2^n \times 2^n$ nodes, the full triangular lattice would have $3 \times 2^n \times 2^n = 3 \cdot 4^n$ springs, therefore using (S2) above,

$$G'_{\rm aff} = G'_{\rm aff,full} \times \frac{N_{\rm spring}}{3 \cdot 4^n} = \frac{\sqrt{3}}{4}k\frac{6(3^m - 2^m)4^{n-m}}{3 \cdot 4^n} = \frac{\sqrt{3}}{2}\left(\frac{3^m - 2^m}{4^m}\right)k \tag{S6}$$

which is the expression used in the main text.

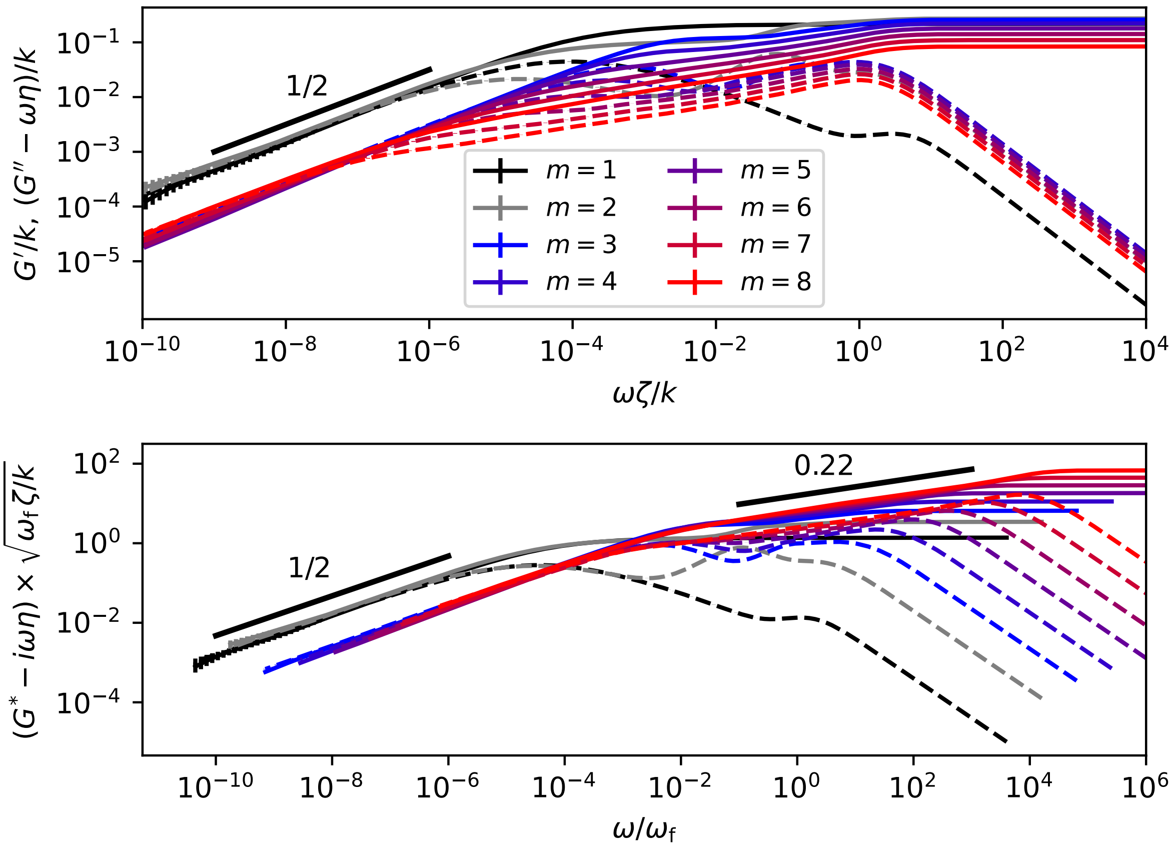


Figure S1: Raw (upper panel) and collapsed (lower panel) viscielastic spectra for $n = 10$ and the $m$ given in the legend. This extends the equivalent plot in the main text by the inclusion of the curves for $m = 1$ (black) and $m = 2$ (grey), which as shown, obey the same scaling and collapse as the $m > 3$ data (blue to red), but collapse onto a distinct master curve.

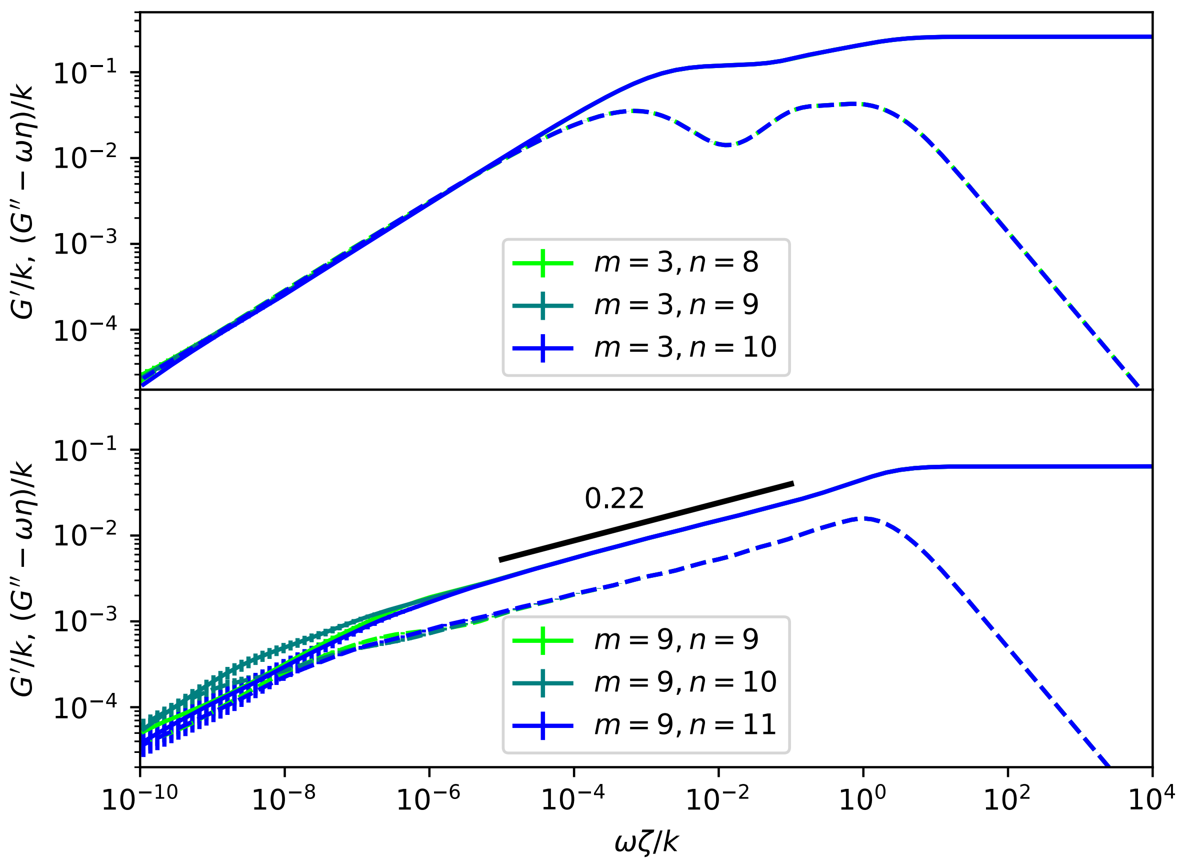


Figure S2: Viscoelastic spectra for $m = 3$ (upper panel) and $m = 9$ (lower panel) for a range of system sizes $n$, where the total system size is $2^n \times 2^n$ nodes. $G'(\omega)$ is plotted as solid lines and $G''(\omega)$ less the fluid contribution $\omega\eta$ as dashed lines. The slope of the intermediate frequency regime is annotated in the lower panel.

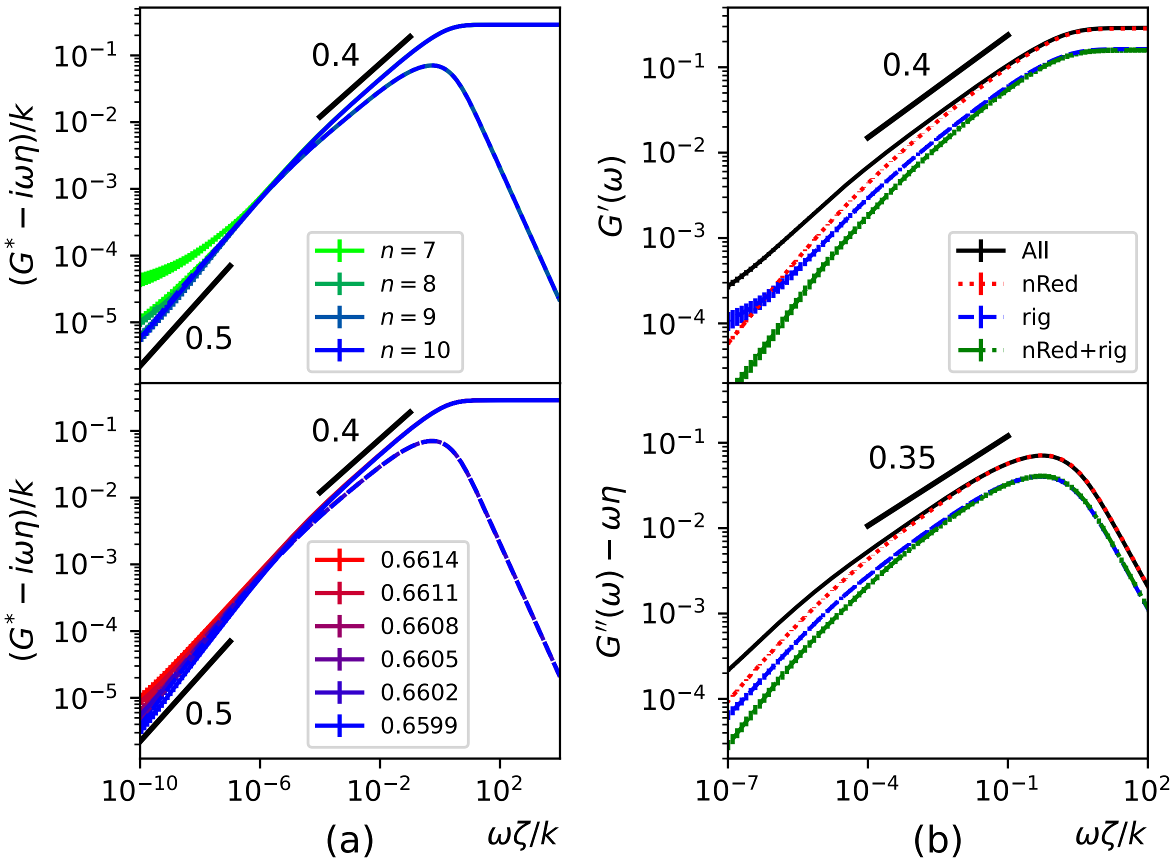


Figure S3: Viscoelastic spectra for bond–diluted triangular lattices. (a) Varying system size $2^n \times 2^n$ for $p = 0.6608$ (top) and varying $p$ for $n = 9$ (bottom). (b) $G'(\omega)$ (top) and the network contribution to $G''(\omega)$ (bottom) for the full network ('All'), redundant bonds removed ('nRed'), rigid cluster only ('rig'), and rigid cluster without redundant bonds ('nRed+rig'), as determined by the pebble game method. Data shown for $p = 0.6608$ and $n = 7$. In all panels the thick black line segments have the annotated slope.

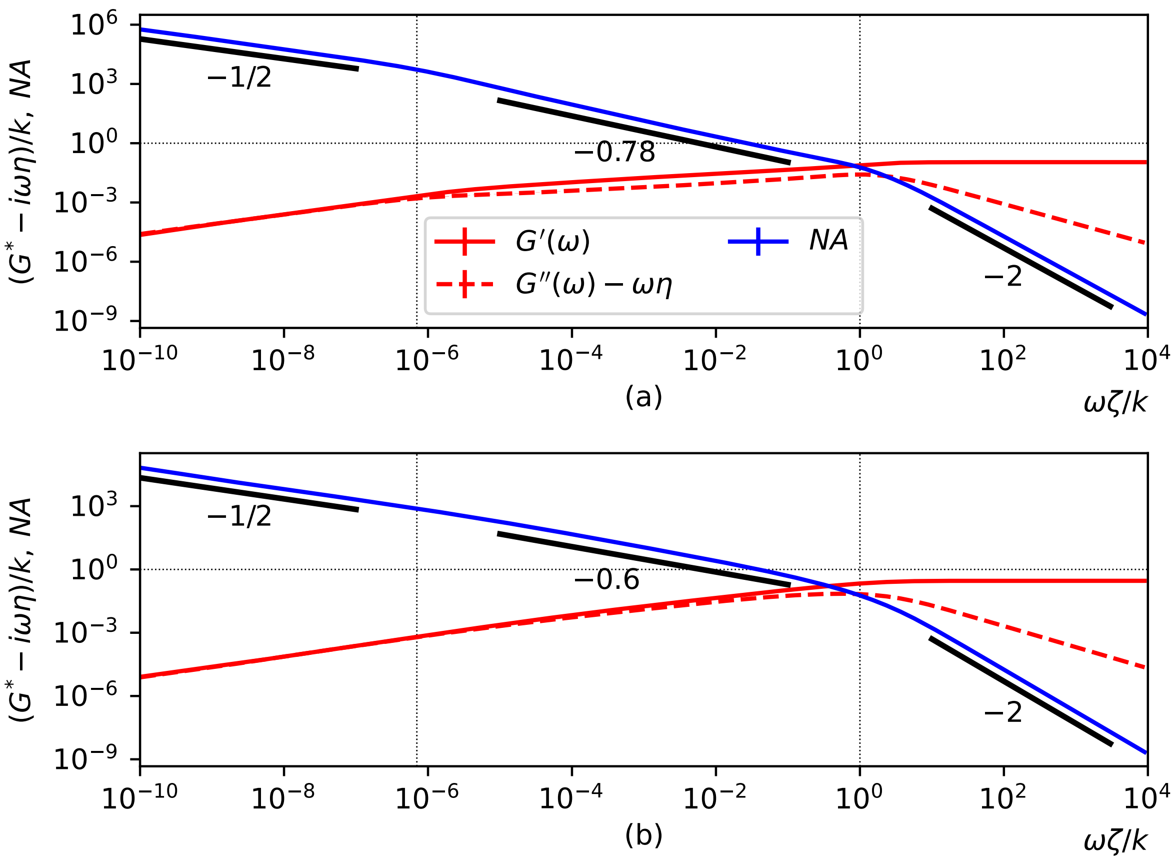


Figure S4: The non–affinity metric $\mathrm{NA} = \frac{1}{Na^2\gamma^2}\sum_\alpha \sum_{i=x,y} \left| u_i^\alpha - u_i^{\alpha,\mathrm{aff}} \right|^2$ averaged over nodes $\alpha = 1 \ldots N$ for (a) a Sierpinski fractal network with $m = 7$ and (b) a bond–diluted network with $p = 0.6608$, close to the percolation transition. In both cases the system size was $2^n \times 2^n$ nodes with $n = 10$. The network contribution to the viscoelastic spectra $G^*(\omega) - i\omega\eta$ is plotted on the same axes in both cases. The short black line segments alongside the NA data have the annotated slopes. In the expression for $NA$, $a$ is the mean lattice spacing, $\gamma$ is the magnitude of the strain, and $\mathbf{u}^{\alpha,\mathrm{aff}}$ is the affine prediction for the displacement of node $\alpha$.

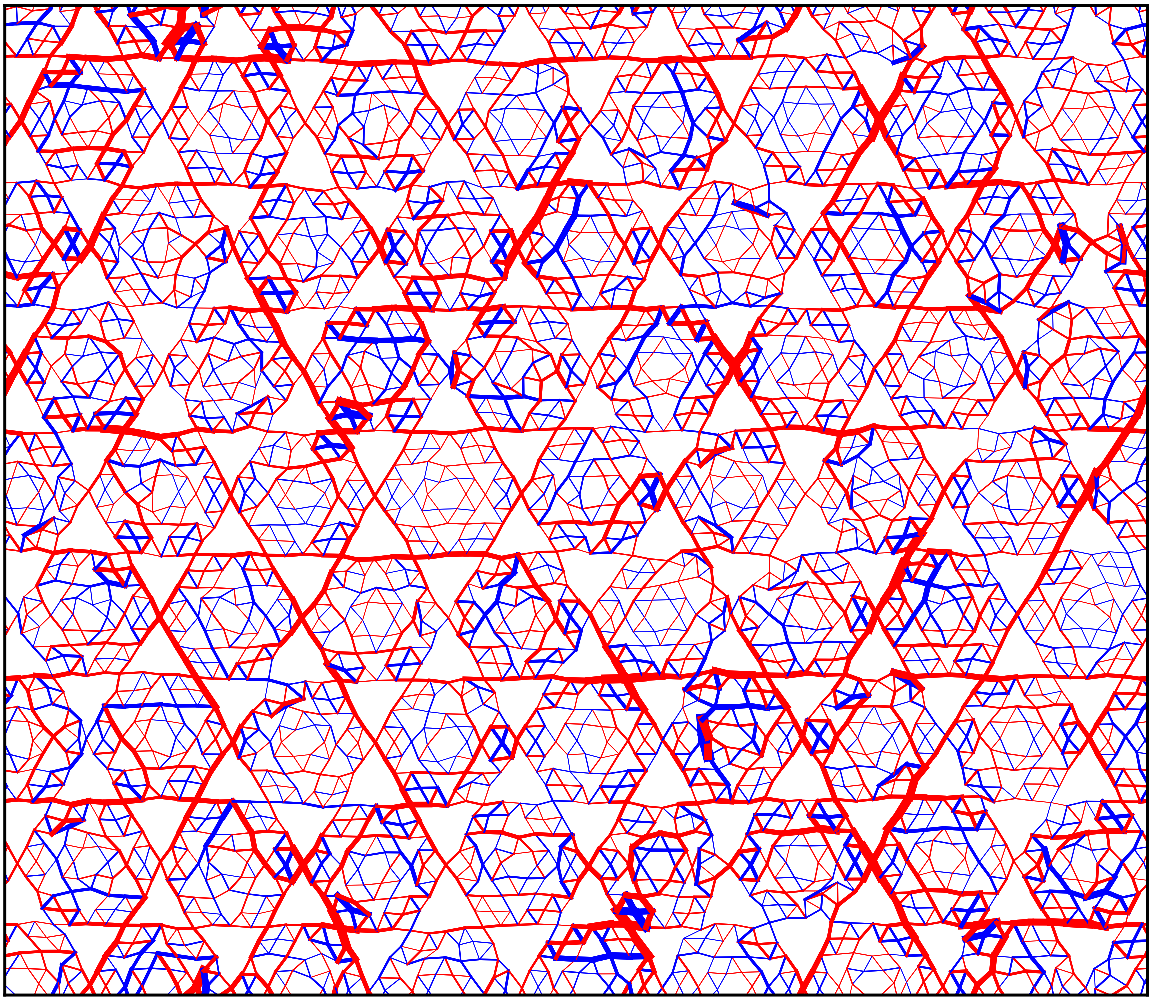

Figure S5: Example of a network with internal stresses for $n = 6$, $m = 3$, and $\Lambda = 0.05$. Springs under tension (compression) are colored red (blue), with a thickness proportional to the magnitude of the tension/compression.

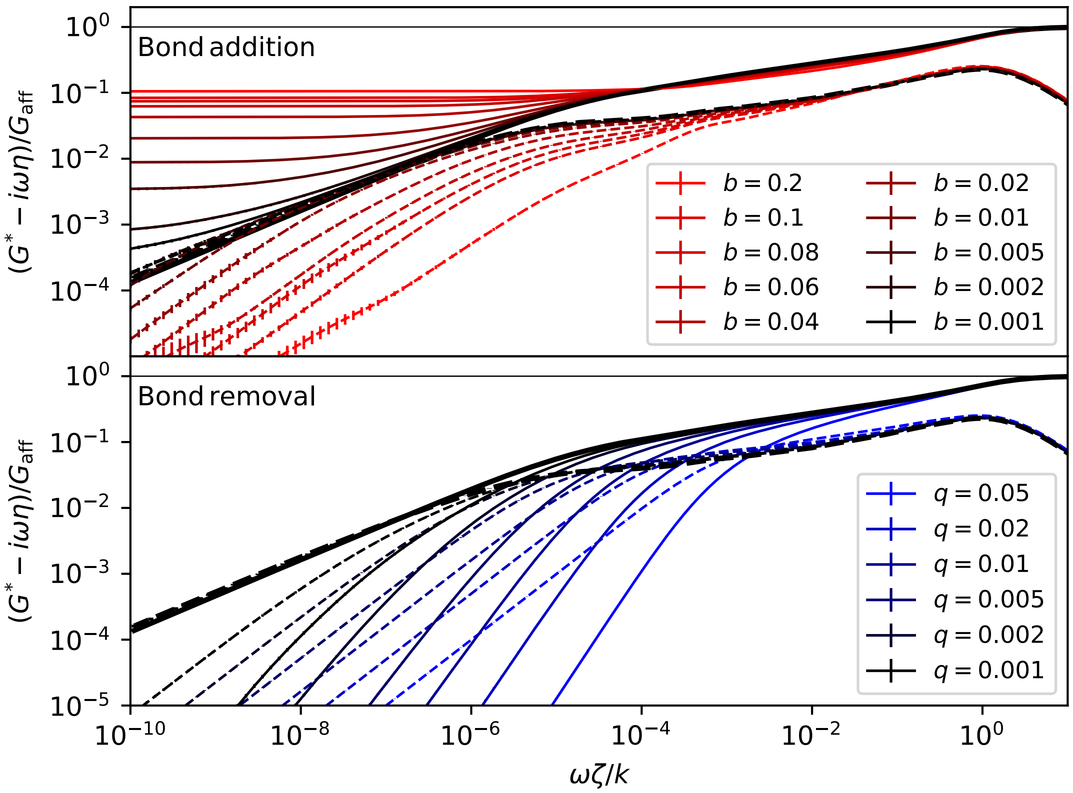


Figure S6: Effect of adding (top) or removing (bottom) bonds for networks with $n = 10$ and $m = 6$. Solid lines correspond to $G'(\omega)$, dashed lines to $G''(\omega)$, and the baseline case with no bonds added or removed is shown in thick black. Bonds were added to the uniform triangular lattice with probability $b$, unless a spring already existed between the same two nodes. Bonds were removed from the baseline fractal lattice with a probability $q$ per bond. The vertical axes have been scaled by the affine prediction $G_{\rm aff}$ for $G'$ as given in the main text.
